# Supplementary material for: Assessing differentially private deep learning with Membership Inference
Source: arXiv:1912.11328 source file (2020-05-26)
Supplement: Supplementary file 1 [file appendix.tex]

\section{Appendix}
\label{sec:append}
\subsection{Hyperparameters for experiments}
\label{app:hyperparam}
To compute the CIFAR-10 target model baseline results of Figure~\ref{fig:cifar-mi-non-private-baseline}, we trained the target model for $100$ epochs with batch size $128$, Adam optimizer, $\text{learning rate}=0.001$ and $\text{learning rate decay}=10^{-7}$. The MI attack was performed with $\abs{\text{shadow models}}=20$ since no change in results occurred when $\abs{\text{shadow models}}>20$.

To compute the MNIST target model baseline results of Figure~\ref{fig:mnist-mi-non-private-baseline} we trained the target model for $15$ epochs with $\text{learning rate}=0.001$ and $\text{learning rate decay}=10^{-7}$. 
Since we drastically reduced the data set size over our experiment we adjusted the batch size according to Table~\ref{tab:mnist-batchsize}. The MI attack was performed with $\abs{\text{shadow models}}=10$ since no change in results occurred when $\abs{\text{shadow models}}>10$.
\begin{table}[ht]
	\centering
	\caption{Chosen batch size for MNIST in Figure~\ref{fig:mnist-mi-non-private-baseline}}
	\label{tab:mnist-batchsize}
	\begin{tabular}{@{}ll@{}}
		\toprule
		$n$ & Batch Size \\ \midrule
		$10,000$  &  $100$  \\
		$5,000$ & $50$ \\
		$2,500$ & $25$ \\
		$1,000$ & $10$ \\
		$500$ &  $5$  \\ 
	    $300$ &  $3$  \\
	    $100$ &  $1$  \\
	    $50$  &  $1$  \\\bottomrule
	\end{tabular}
\end{table}

\begin{table}[ht]
	\centering
	\caption{Hyperparameter setting for Skewed Purchases.}
	\label{tab:purchases:hyperparameters}
	\begin{tabular}{@{}ll@{}}
		\toprule
		Parameter & Value \\ \midrule
		batch size  & 100   \\
		cost function & cross entropy \\
		$\alpha$       & $0.001$ \\
		$\alpha$-decay & 1e-5  \\
		epoch       & 200   \\ 
		$\abs{\text{shadow models}}$ & 20 \\\bottomrule
	\end{tabular}
\end{table}
\begin{table}[ht]
	\centering
	\caption{Hyperparameter setting to train DP target models on Skewed Purchases with $n=10,000$ and $200$ epochs}
	\label{tab:purch-hyperparameter-10000}
	\begin{tabular}{@{}lccccc@{}}
		\toprule
		Parameter & $\eps=0.9$ & $\eps=1.8$ & $\eps=2.4$ & $\eps=3.7$ & $\eps=8.4$\\ \midrule
		Batch Size  & $100$   & $100$ &  $100$ & $100$ & $100$\\
		Lot Size & $100$  & $100$  & $100$ & $100$ & $100$\\
		Learning Rate & $0.001$ & $0.001$ & $0.001$ & $0.001$ & $0.001$\\
		Norm Bound & $4$  & $4$ & $4$ & $4$ & $4$\\
		$\abs{\text{shadow models}}$ & $20$   &  $20$ & $20$ & $20$ & $20$\\
		\sgm      & $16$   &  $8$ & $6$ & $4$ & $2$\\\bottomrule
	\end{tabular}
\end{table}

\subsection{Imbalance of provided Datasets}
\label{app:imbalance}
The Texas Hospitals Stays and Purchases Shopping Carts datasets provided by Shokri et al.~are unbalanced in terms of records per class. This is shown in Figures~\ref{fig:unbalanced:purch} and~\ref{fig:unbalanced:th}. The imbalance affects mainly the target test accuracy.

\begin{figure}[h]
	\centering
	\includegraphics[width=0.95\linewidth]{./fig/shokri_purchases_dataset_distribution.pdf}
	\caption{The Quantity of records per Label for the Purchases Shopping Cart Dataset}
	\label{fig:unbalanced:purch}
\end{figure}

\begin{figure}[h]
	\centering
	\begin{subfigure}{0.5\linewidth}
		\includegraphics[width=1\linewidth]{./fig/shokri_th_dataset_distribution_100.pdf}
		\caption{$\var{C}=100$}
	\end{subfigure}%
	\begin{subfigure}{0.5\linewidth}
		\includegraphics[width=1\linewidth]{./fig/shokri_th_dataset_distribution_150.pdf}
		\caption{$\var{C}=150$}
	\end{subfigure}
	\begin{subfigure}{0.5\linewidth}
		\includegraphics[width=1\linewidth]{./fig/shokri_th_dataset_distribution_200.pdf}
		\caption{$\var{C}=200$}
	\end{subfigure}%
	\begin{subfigure}{0.5\linewidth}
		\includegraphics[width=1\linewidth]{./fig/shokri_th_dataset_distribution_300.pdf}
		\caption{$\var{C}=300$}
	\end{subfigure}
	\caption{The Quantity of records per Label for the Texas Hospital Stays Dataset}
	\label{fig:unbalanced:th}
\end{figure}

\subsection{PCA against MI}
\label{app:pca}

In Section~\ref{sec:prel:mi} we showed that training data set size $n$ influences MI Precision. In the case of Texas Hospital Stays we directly observe that the dataset is of high dimensionality (thousands of features). Thus, in practice, Principal Component Analysis (PCA) or and alternative feature reduction algorithm would likely be applied to reduce the input dimensions before training a neural network. Now of particular interest to the practical relevance of our evaluation is whether the MI precision in this dataset is solely due to excessive dimensionality. Figure~\ref{fig:eval:th:pca} depicts the development of original MI precision over the number of principal components. Note that the decrease in the explained variance ratio also results in a decrease in target model test accuracy since the training data is less detailed after PCA. It is notable that PCA does not significantly lower MI Precision and thus dimensionality is not a dominant driver for MI.

\begin{figure}[h]
	\centering
	\includegraphics[width=0.7\linewidth]{./fig/ldp_mi_precision_over_pca_dimensions_normal_shadows}
	\caption{PCA effect on Texas Hospital Stays MI precision}	
	\label{fig:eval:th:pca}
\end{figure}

\subsection{Dataset size and class balance against MI}
\label{app:mi}
\begin{figure}[h]
	\centering
		\includegraphics[width=0.7\linewidth]{vldb_mi_cifar_baseline_summary.pdf}
		\caption{Target model accuracy and MI precision for CIFAR-10 over $n$.}
		\label{fig:cifar-mi-non-private-baseline}
\end{figure}

\begin{figure}[h]
	\centering
		\includegraphics[width=0.7\linewidth]{vldb_mi_unbalanced_cifar.pdf}%
		\caption{MI precision for CIFAR-10 over varying levels of imbalance. Imbalance is created by keeping only a fraction of the images for \textit{cats} in the training data for target and shadow models.}
		\label{fig:cifar-mi-unbalance}
\end{figure}
Findings by Shokri et al.~\cite{shokri2017} indicate that MI becomes less precise, if more target model training data $n$ is used. Hence, in practice the effectiveness of MI might already be prevented by using a large amount of training data. For illustration we evaluate the CIFAR-10 dataset under MI to analyze the impacts of varying $n$. For this experiment, we pre-train the target model on CIFAR-100, considering it a public dataset, before performing training on the assumed sensitive CIFAR-10 dataset\footnote{\tiny Publicly available: \url{https://www.cs.toronto.edu/~kriz/cifar.html}}. This approach has been initially proposed by Abadi et al.~\cite{abadi2016}.
We further train the target model on subsets of the original CIFAR-10 training set with $n \in \{2500, 5000, 10000, 15000\}$ to test the effect of $n$ on MI. 
The mean MI precision over all classes and the train and test accuracies of the target model for different $n$ are depicted in Figure~\ref{fig:cifar-mi-non-private-baseline}. 
The figure underlines that decreasing amounts of training data result in a growing train-test-gap (i.e., gap between train and test accuracy) that correlates with the increase in MI precision.
The MI precision curve converges at a MI precision of$\approx0.7$ for $n=15,000$. Thus, the MI attack is also functioning even when $n$ is increased.

%We observed that instances of cats were prone to higher MI precision than instances from other class distributions of the CIFAR-10 data set. Consequently, the average MI precision can be misleading, especially when the training dataset is unbalanced w.r.t.~the vulnerable class. 
Furthermore, we assume learning on unbalanced data, i.e., when there is a significant difference in the numbers of instances per class, especially reasonable when dealing with sensitive classes for which it might be harder to gather as much training data as for non-sensitive classes. To illustrate the MI in this case, we fix one class $Y_i$ that has considerably less instances in the training set compared to all other classes. Hence, the dataset \subsup{\cali{D}}{}{train} is only unbalanced w.r.t.~$Y_i$, and balanced for all other classes. With this setup, we intentionally make one class (more) vulnerable to MI as we keep its number of instances small. Thus, if the instances per class for all $Y_k,k\ne i$ are increased, we expect the train-test gap to get smaller since only one class is likely to overfit. In consequence the utility-privacy trade-off to improve as more data implies higher noise robustness.
We introduced an imbalance to the CIFAR-10 dataset by continuously decreasing the ratio of training instances of class $Y_i$, depicting cats, compared to training instances of other classes, from $100\%$ -- $1\%$. The results in Figure~\ref{fig:cifar-mi-unbalance} demonstrate the effect of different ratios of imbalance on MI precision and target model test accuracy. %While protection with DP is especially effective when the factor of imbalance is low, this benefit sharply decreases with growing imbalance among classes.
